# Supplementary material for: Oracle Complexity Separation in Convex Optimization
Source: arXiv:2002.02706 source file (2022-03-11)
Supplement: Supplementary file 1 [file appendix.tex]

%\onecolumn
\iffalse
\begin{center}
\vspace*{1pt}
{\Large\bf{APPENDIX}}

% \vspace*{10pt}
% {\Large\bf{Adaptive Catalyst for Smooth Convex Optimization}}
\end{center}
% \vspace*{-4pt}
%\hline
\noindent\rule{\textwidth}{1pt}
\appendix
\fi

\section{\gav{Theoretical explanation the results of the experiments}}\label{mot_ex}
\gav{In this section, we present theoretical arguments which support the findings of the experiments described in Section~\ref{exp}.}

\subsection{Kernel SVM}\label{app:svm}
Let us consider the following function
$$f(x) = \frac{1}{m}\sum_{k=1}^m f_k(\left\langle A_k, x \right\rangle) + \frac{1}{2}\left\langle x,Cx \right\rangle,$$
where the matrix $C$ is equal to $\lambda K$ in the notation of the previous section and $A_k$ is equal to $b_kK$ in the notation of the previous section.
We assume that $|f_k''(y)| = O(1/\epsilon)$,  matrix $A = [A_1,...,A_m]^{\top}$ has $ms$ nonzero elements, $\max_{k=1,...,m} \|A_k\|_2^2 = O(s)$, where $1\ll s \le n$ and $C$ is positive semidefinite  matrix,\footnote{Here an below we also assume after `semidefinite' that valuable part of the spectrum of dens matrix $C$ lies in a small (right) vicinity of zero point on real line.} with $\lambda_{\max}(C)\le 1/(\varepsilon m)$. 
Fast Gradient Method \gav{(FGM)} \cite{nesterov2018lectures} requires $$O\left(\sqrt{\frac{\left(s/\varepsilon + \lambda_{\max}(C)\right)R^2}{\varepsilon}}\right)$$
iterations with the complexity of each iteration\footnote{To obtain the part of the complexity $O(ms)$ one should use special representation of matrix $A$ in the memory -- adjacency list. The same requirements take place for other algorithms.}
$$O\left(ms + n^2\right).$$
For proposed in this paper approach we have
$$\tilde{O}\left(\sqrt{\frac{ \lambda_{\max}(C)R^2}{\varepsilon}}\right)$$
iterations of FGM for the second term in target function with the complexity of each iteration
$$O(n^2)$$
and
$$\tilde{O}\left(\sqrt{\frac{\left(ms/\varepsilon \right)R^2}{\varepsilon}}\right)$$
iterations of variance reduction algorithm \cite{allen2017katyusha} with the complexity of each 
$$O(s).$$

We combine all these results in the table below. From the table one can conclude that 
 since $s\gg 1$, $\lambda_{\max}(C)\le 1/(\varepsilon m)\ll s/\varepsilon$, then 
our approach has better theoretical complexity.
\begin{center}
\begin{table}[H]
\label{table_0}
\begin{tabular}{|c|c|c|ll}
\cline{1-3}
 Algorithm  & Complexity&  Reference&   &  \\ \cline{1-3}
FGM & $ O\left(\frac{R}{\varepsilon}\sqrt{s}\left(ms + n^2\right)\right) $ & \cite{nesterov2018lectures} &  &  \\ \cline{1-3}
% coordinate FGM & $ O\left(n\sqrt{\frac{R^2}{\varepsilon}}\left(p + n\right)\right) $ & \cite{nesterov2017efficiency} &  &  \\ \cline{1-3}
Our approach & $ \tilde{O}\left(\frac{R}{\varepsilon}\sqrt{ms}\cdot s\right) + \tilde{O}\left(\sqrt{\frac{\lambda_{\max}(C)R^2}{\varepsilon}}\cdot n^2\right) $ & this paper &  &  \\ 
 \cline{1-3}
% Local SGD & $1$ & $2$ &  &  \\
% \cline{1-3}
\end{tabular}
\end{table}
\end{center}

\subsection{Soft-max plus quadratic form}\label{app:soft}
Let's consider the following function
$$
f(x) = \log\left(\sum_{k=1}^p \exp \left(\left\langle A_k, x \right\rangle\right)\right) + \frac{1}{2} \|G x\|_2^2 \rightarrow \min_{x \in \mathbb{R}^n}.
$$
We introduce matrix $A = [A_1,...,A_p]^{\top}$, is such that $\max_{ij} |A_{ij}| = O(1)$, $\max_{j=1,...,n} \|A^{<j>}\|_2^2 = O(n)$ and $A$ has $O(ps)$ nonzero elements; $G^2$ is positive semidefinite  matrix with $\lambda_{\max}(G^2) = O(n)$ and $\frac{1}{n}\sum_{i=1}^n \sqrt{G^2_{ii}} = O(1)$.

Fast Gradient Method \cite{nesterov2018lectures} requires $$O\left(\sqrt{\frac{\left(\max_{j = 1,..., n} \|A^{<j>}\|_2^2 + \lambda_{\max}(G^2)\right)R^2}{\varepsilon}}\right)$$
iterations with the complexity of each iteration
$$O\left(ps + n^2\right).$$ Coordinate Fast Gradient Method \cite{nesterov2017efficiency}
requires $$O\left(n\sqrt{\frac{\left(\max_{ij} |A_{ij}|^2+ \left(\frac{1}{n}\sum_{i=1}^n \sqrt{G^2_{ii}} \right)^2\right)R^2}{\varepsilon}}\right)$$
iterations with the complexity of each iteration\footnote{Here one should use a following trick in recalculation of $\log\left(\sum_{k=1}^p \exp \left(\left\langle A_k, x \right\rangle\right)\right)$ and its gradient (partial derivative). From the structure of the method we know that $x^{new} = \alpha x^{old} + \beta e_i$, where $e_i$ is $i$-th orth. So if we've already calculate $\left\langle A_k, x^{old} \right\rangle$ then to recalculate $\left\langle A_k, x^{new} \right\rangle = \alpha\left\langle A_k, x^{old} \right\rangle + \beta [A_k]_i$ requires only $O(1)$ additional operations independently of $n$ and $s$.}
$$O\left(p + n\right).$$
For proposed in this paper approach we have
$$\tilde{O}\left(\sqrt{\frac{\left(\max_{j = 1,..., n} \|A^{<j>}\|_2^2 + \lambda_{\max}(G^2)\right)R^2}{\varepsilon}}\right)$$
iterations of FGM for the first term in target function with complexity of each iteration
$$O(ps)$$
and
$$\tilde{O}\left(n\sqrt{\frac{ \left(\frac{1}{n}\sum_{i=1}^n \sqrt{G^2_{ii}} \right)^2R^2}{\varepsilon}}\right)$$
iterations of coordinate FGM for the second term in target function with complexity of each iteration
$$O(n).$$

We combine all these results in the table below. From the table one can conclude that if $n \ll p$, $s\ll \min\left\lbrace n^2/p,\sqrt{n}\right\rbrace$, then our approach has better theoretical complexity.
\begin{center}
\begin{table}[H]
\label{table_1}
\begin{tabular}{|c|c|c|ll}
\cline{1-3}
 Algorithm  & Complexity&  Reference&   &  \\ \cline{1-3}
FGM & $ O\left(\sqrt{\frac{nR^2}{\varepsilon}}\left(ps + n^2\right)\right) $ & \cite{nesterov2018lectures} &  &  \\ \cline{1-3}
coordinate FGM & $ O\left(n\sqrt{\frac{R^2}{\varepsilon}}\left(p + n\right)\right) $ & \cite{nesterov2017efficiency} &  &  \\ \cline{1-3}
Our approach & $ \tilde{O}\left(\sqrt{\frac{nR^2}{\varepsilon}}\cdot ps\right) + \tilde{O}\left(n\sqrt{\frac{R^2}{\varepsilon}}\cdot n\right) $ & this paper &  &  \\ \cline{1-3}
% Local SGD & $1$ & $2$ &  &  \\
% \cline{1-3}
\end{tabular}
\end{table}
\end{center}

\section{Proof of the main result}\label{App:proof}

The proof of the main result \gav{(Theorem~\ref{main_theo})} consists of four steps:
\begin{enumerate}
    \item Estimating the number of iterations of the inner method $\mathcal{M}_{inn}$.
    \item Estimating the number of iterations of  Algorithm~\ref{alg:gradient_for_composite}.
    \item Estimating the number of iterations of Algorithm~\ref{alg:MS} with the restarting strategy as in Algorithm~\ref{Alg:rest_str_MS}.
    \item Obtaining a final estimate of the number of iterations of oracles $O_f$ and $O_g$ based on estimates from steps $1-3$.
\end{enumerate}

\subsection{Step 1.}

On each iteration of  Algorithm~\ref{alg:gradient_for_composite} we need to solve the problem
\begin{equation}
    \min\limits_{v \in \mathbb{R}^n}\varphi(v) :=  \left\langle \nabla h(v^k), v - v^k \right\rangle 
+ g(v)  + \tfrac{L}{2}\|v-v^0\|_2^2   + \tfrac{L_h}{2} \|v - v^k\|_2^2.
    \label{aux_problem}
\end{equation}

Applying the method $\mathcal{M}_{inn}$ to~\eqref{aux_problem} with $\alpha = L + L_h$ we obtain that in $N_{\mathcal{M}}(\tilde{\varepsilon}) = O\left(\tfrac{\tau_{g}}{\sqrt{L + L_h}}\ln\tfrac{C ||v^0-v^{\ast}||_2^2}{\tilde{\varepsilon}} \right)$ Oracle calls we can find $v^{N_{\mathcal{M}}(\tilde{\varepsilon})}$ such that  
\begin{equation}
    \label{varphi_est}
	\E (\varphi(v^{N_{\mathcal{M}}(\tilde{\varepsilon})}) - \varphi(v^{\ast})) \leq \tilde{\varepsilon}.
\end{equation}
Since $\varphi(v^{N_{\mathcal{M}}(\tilde{\varepsilon})}) - \varphi(v^{\ast}) \geq 0$, with an arbitrary $\tilde{\delta}\in(0,1)$ we can apply the Markov inequality:
\begin{equation*}
	\PP \left(\varphi(v^{N_{\mathcal{M}}(\tilde{\delta}\tilde{\varepsilon})}) - \varphi(v^{\ast}) \geq \tilde{\varepsilon} \right) \leq \tfrac{\E (\varphi(v^{N_{\mathcal{M}}(\tilde{\delta} \tilde{\varepsilon})}) - \varphi(v^{\ast}))}{\tilde{\varepsilon}} \leq  \tilde{\delta}.
\end{equation*}

We have shown that with probability at least $1 - \tilde{\delta}$ in
$$N_{\mathcal{M}}(\tilde{\delta}\tilde{\varepsilon}) = O\left(\tfrac{\tau_{g}}{\sqrt{L + L_h}}\ln\tfrac{C ||v^0-v^{\ast}||_2^2}{\tilde{\delta} \tilde{\varepsilon}} \right)$$
Oracle calls we can find $\hat{v}$ such that $\varphi(\hat{v}) - \varphi(v^{\ast}) \leq \tilde{\varepsilon}$.
Since $\varphi(\cdot)$ is $L+L_h$ strongly convex, we have

$$
    \tfrac{L+L_h}{2}||\hat{v} - v^{\ast}||_2^2 \leq \varphi(\hat{v}) - \varphi(v^{\ast}) \leq \tilde{\varepsilon}.
$$
Moreover, since $\varphi(\cdot)$ is $L_g$-smooth and $\nabla \varphi(v^{\ast}) = 0$ 
$$
    ||\nabla \varphi(\hat{v}) ||_2 \leq L_g||\hat{v} - v^{\ast}||_2.
$$
Using these two inequalities, we obtain 
 \begin{eqnarray*}
     \left\langle  \nabla \varphi(\hat{v}), \hat{v} - v^{\ast} \right\rangle  \leq   ||  \nabla \varphi(\hat{v})||_2 \cdot || \hat{v} - v^{\ast}  ||_2 \leq L_g||\hat{v} - v^{\ast}||_2^2 \leq L_g \tfrac{2\tilde{\varepsilon}}{L+L_h}.
 \end{eqnarray*}
 This leads to the following lemma
 \begin{lem}
 \label{inn_est}
 Applying the method $\mathcal{M}_{inn}$ to~\eqref{aux_problem} we have that with probability at least $1 - \tilde{\delta}$ in $N_{\mathcal{M}}(\tilde{\varepsilon}) = O\left(\tfrac{\tau_{g}}{\sqrt{L + L_h}}\ln\tfrac{2C L_g ||v^0-v^{\ast}||_2^2}{\tilde{\delta}\tilde{\varepsilon}(L+L_h)} \right)$ Oracle calls we can find $\hat{v}$ such that 
 \begin{align}
  \label{inex_sol}
    \left\langle  \nabla \varphi(\hat{v}), \hat{v} - v^{\ast} \right\rangle &\leq \tilde{\varepsilon},\\
     \label{inex_sol_arg}
    ||\hat{v} - v^{\ast}||^2_2 &\leq \tfrac{1}{L_g}\tilde{\varepsilon}.
    \end{align}
 \end{lem}
% \pd{The first part of definition does not give the same definition of inexactness as in the Definition 1 in Appendix. Thus, we can't apply Theorem 2.}

\subsection{Step 2.}
To estimate the number of iterations of Algorithm~\ref{alg:gradient_for_composite} note that the MS condition
\begin{eqnarray*}
    \|\nabla F_{L, \zeta^0 } (\hat{\zeta}^k)\|_2 \leq \tfrac{L}{2} \|\hat{\zeta}^k - \zeta^0\|_2 
\end{eqnarray*}
instead of the exact solution $\zeta^{\ast}$ of the auxiliary problem in the Algorithm~\ref{alg:MS}, for which
\begin{eqnarray*}
    \|\nabla F_{L, \zeta^0}  (\zeta^{\ast})\|_2 = 0,
\end{eqnarray*}
allows to search inexact solution $\hat{\zeta}^k$. 

Since the function $F_{L, \zeta^0}(\cdot)$ is $(L+L_f)$-smooth, we have
\begin{equation}
\label{eq:1}
    || \nabla F_{L, \zeta^0}(\hat{\zeta}^k)||_2 \leq  (L+L_f)||\hat{\zeta}^k - \zeta^{\ast}||_2.
\end{equation}
Using the triangle inequality we have 
\begin{equation}
  \label{eq:2}
    ||\zeta^0 - \zeta^{\ast}||_2 - ||\hat{\zeta}^k -  \zeta^{\ast}||_2 \leq || \hat{\zeta}^k - \zeta^0 ||_2.  
\end{equation}
Since r.h.s. of the inequality~\eqref{eq:1} coincide with the r.h.s. of the M-S condition and l.h.s. of the inequality~\eqref{eq:2}
coincide with the l.h.s. of the M-S condition up to a multiplicative factor $L/2$, one can conclude that if the inequality 
\begin{equation}
\label{inner_est}
      ||\hat{\zeta}^k - \zeta^{\ast}||_2 \leq \tfrac{L}{3 L + 2L_{f}}  ||\zeta^0 -\zeta^{\ast}||_2
\end{equation}
holds, the M-S condition holds too, where $\zeta^0$ is a starting point.

We assume that on each iteration of the Algorithm~\ref{alg:gradient_for_composite} we solve an auxiliary problem~\eqref{algGMCO_aux} in the sense of~\eqref{inex_sol}. Then, we provide the following convergence rate theorem for the Algorithm \ref{alg:gradient_for_composite}:

\begin{theorem}\label{Th:gradient_for_composite}
Assume that $\frac{\mu + L}{2L_h} \leq 1$. After $N$ iterations of Algorithm \ref{alg:gradient_for_composite} we have
\begin{equation*}
\begin{aligned}
F_{L, \zeta^0}(\zeta^N) - F_{L, \zeta^0}(\zeta^{\ast}) &\leq \exp\left(-\tfrac{N(\mu + L)}{4L_h}\right) (F_{L, \zeta^0}(\zeta_0) - F_{L, \zeta^0}(\zeta^{\ast})) + \tfrac{4L_h}{\mu + L}\tilde{\varepsilon}, \\
\tfrac{1}{2}||\zeta^{\ast} - \zeta^N||^2_2 &\leq \tfrac{L_h}{2(\mu + L)} ||\zeta^{\ast} -  \zeta_0||^2_2 + \tfrac{4L_h}{(\mu + L)^2}\tilde{\varepsilon}.
\end{aligned}
\end{equation*}

\
\end{theorem}

\textit{The proof of this \gav{auxiliary} Theorem is given in \gav{Section~\ref{GMCO}}.}

Now we consider the function $F_{L, \zeta^0}(\cdot)$ as an $L$-strongly convex function, not taking $\mu$ into account. From Theorem~\ref{Th:gradient_for_composite} we obtain that 
\begin{equation*}
    F_{L, \zeta^0}(\zeta^N) - F_{L, \zeta^0}(\zeta^{\ast} )   \leq \tfrac{L_{h}||\zeta^0 - \zeta^{\ast}||_2^2}{2}\exp\left( \tfrac{-N L } {4L_h}\right) + \tfrac{4L_h}{L}\tilde{\varepsilon}.
\end{equation*}
From strong convexity of $F_{L, \zeta^0}(\cdot)$, the following inequality holds. \cite{nesterov2018lectures}
\begin{eqnarray*}
 \tfrac{L}{2}||\hat{\zeta}^N- \zeta^{\ast}||^2_2 
  \leq F_{L, \zeta^0}(\hat{\zeta}^N) - F_{L, \zeta^0}(\zeta^{\ast} ) .
\end{eqnarray*}
Thus, for condition~\eqref{inner_est} to be satisfied, it is necessary that
\begin{equation*}
     \tfrac{L_{h}||\zeta^0 - \zeta^{\ast}||_2^2}{2}\exp\left( \tfrac{-N L } {L_h}\right) + \tfrac{4L_h}{L}\tilde{\varepsilon} \leq \tfrac{L^3}{2(3 L + 2L_{f})^2} ||\zeta^0 - \zeta^{\ast}||^2_2.
\end{equation*}
Equating each term of l.h.s. to half of the r.h.s. we obtain that the number of iterations of Algorithm~\ref{alg:gradient_for_composite} is 
\ai{$$
    N_{\text{GMCO}} \overset{def}{=} O\Bigl( \tfrac{L_h}{L} \ln\left(\tfrac{(3 L + 2L_{f})^2 L_h}{L^3} \right) \Bigr)
$$}
and $\tilde{\varepsilon} = \varepsilon_{\mathcal{M}} \overset{def}{=} \tfrac{L^4}{8L_h(3 L + 2L_{f})^2} ||\zeta^0 - \zeta^{\ast}||^2_2$.

Assuming that on each iteration of Algorithm~\ref{alg:gradient_for_composite} we solve the auxiliary problem~\eqref{aux_problem} with probability at least $1 - \delta_{\text{MS}} / N_{\text{GMCO}}$  in the sense of~\eqref{inex_sol} with $\tilde{\varepsilon} = \varepsilon_{\mathcal{M}}$, using the union bound over all $ N_{\text{GMCO}}$ iterations we obtain 
\begin{lem}
   In $N_{\text{GMCO}}$ iterations of  Algorithm~\ref{alg:gradient_for_composite} with probability at least $1 - \delta_{\text{MS}}$ we find $\hat{\zeta}$ such that
   \begin{eqnarray*}
    \|\nabla F_{L, \zeta^0 } (\hat{\zeta})\|_2 \leq \tfrac{L}{2} \|\hat{\zeta} - \zeta^0\|_2.
\end{eqnarray*}
\end{lem}

\subsection{Step 3.}
To estimate the number of iterations of Algorithm~\ref{alg:MS} note that in~\eqref{aux_pr} we apply  Algorithm~\ref{alg:gradient_for_composite} and, according to the stopping criterion of $\text{GMCO}(x^{k+1},F_{L, x^{k+1}})$ obtain $y^{k+1}$ such that 
\begin{equation}
\label{MS_cond}
  \|\nabla F_{L, x^{k+1}} (y^{k+1})\|_2 \leq \tfrac{L}{2} \|y^{k+1} - x^{k+1}\|_2.   
\end{equation}

So we can apply the Theorem 3.6 from~\cite{monteiro2013accelerated} for  Algorithm~\ref{alg:MS} and obtain that for all $N \geq 0$
\begin{equation}
\label{eq12}
f\left( {y^N} \right)-f\left( {x^{\ast} } \right)\le \tfrac{R^2}{2A_N },
\quad
\left\| {z^N-x^{\ast} } \right\|_2 \le R,
\end{equation}
where $R \geq \left\| {y^0-x^{\ast} } \right\|_2$. Moreover, from Lemma 3.7 a) of ~\cite{monteiro2013accelerated} for all $N \geq 0$
\begin{equation}
\label{eq14}
A_N \ge \tfrac{N^2}{4L}.
\end{equation} 

Substituting the inequality~\eqref{eq14} into the estimate \eqref{eq12} we obtain that after $N$ iterations of Algorithm~\ref{alg:MS} the following inequality holds. 
 \begin{equation}
 \label{MS_func_est}
     f(y^N) - f(x_\ast) \leq \tfrac{2L||x^0 - x^{\ast}||_2^2}{N^2}.
 \end{equation}
 Thus,  if $\mu = 0$, then the total number of iterations of MS is $T^{\text{c}}_{\text{MS}}(\varepsilon) \overset{def}{=} \sqrt{\tfrac{L||x^0 - x^{\ast}||_2^2}{\varepsilon}}$.
 
 If $\mu > 0$, to recover the acceleration through strong-convexity we need to apply the restarting strategy. 

In light of the definition of strong convexity of $f(\cdot)$ and the estimate ~\eqref{MS_func_est}, we have
 \begin{eqnarray*}
    \tfrac{\mu}{2}||y^N - x^{\ast}||_2 \leq  f(y^N) - f(x^{\ast}) \leq \tfrac{2L}{N^2}||x^0 - x^{\ast}||_2^2.
 \end{eqnarray*}
 In particular, in every $N = N_0 = \sqrt{\tfrac{8L}{\mu}}$ iterations, we can halve the distance $||y^N - x^{\ast}||_2 \leq \tfrac{1}{2}||x^0 - x^{\ast}||_2^2.$ And if we repeatedly invoke $\text{MS}(\cdot, L, N_0)$ $t$ times, each time choosing the initial point $x_0$ as the previous output $y^{N_0}$, then in the last run of $N_0$ iterations, we have 
  \begin{eqnarray*}
     f(y^{N_0}) - f(x^{\ast}) \leq \tfrac{4 L}{2^t N_{0}^2}||x^0 - x^{\ast}||_2^2 = \tfrac{1}{2^{t+1}}||x^0 - x^{\ast}||_2^2.
 \end{eqnarray*}

By choosing $t = \log\left(\tfrac{||x_0 - x^{\ast}||_2^2 \cdot \mu}{\varepsilon} \right)$, we conclude that 
\begin{lem}
\label{MS_res_lem}
     If $f(\cdot)$ is $\mu$-strongly convex w.r.t. $||\cdot||_2$, then after 
     
     $T=T(\varepsilon) \overset{def}{=} \log\left(\tfrac{\mu||\eta_0 - \eta^{\ast}||_2^2}{\varepsilon} \right)$ iterations of the Algorithm~\ref{Alg:rest_str_MS} we obtain some $\eta_T$ such that $f(\eta_T) - f(\eta^{\ast}) \leq \varepsilon$.
\end{lem}

From this lemma we obtain that the total number of iterations of $\text{MS}$ is $T^{\text{sc}}_{\text{MS}}(\varepsilon)\overset{def}{=} O\left(\sqrt{\tfrac{L}{\mu}} \log\left(\tfrac{\mu||\eta_0 - \eta^{\ast}||_2^2}{\varepsilon} \right)\right)$. 

Assume that on each iteration of the Algorithm~\ref{alg:MS} we find $y^{k+1}$ satisfying~\eqref{MS_cond} with probability at least $1-\delta_{\text{MS}}$ with $\delta_{\text{MS}} = \delta / T_{\text{MS}}(\varepsilon)$, where $\delta \in (0,1)$ and
$$
T_{\text{MS}}(\varepsilon) = 
  \begin{cases} 
   T^{\text{SC}}_{\text{MS}}(\varepsilon) & \text{if } \mu \geq 0, \\
   T^{\text{C}}_{\text{MS}}(\varepsilon)       & \text{if } \mu = 0.
  \end{cases}
 $$ 
  
Using the union bound over all iterations of $\text{MS}$ and Lemma~\ref{MS_res_lem} for the strongly convex case, we obtain the following lemma.
\begin{lem}
    If on each iteration of Algorithm~\ref{alg:MS} we find $y^{k+1}$ satisfying~\eqref{MS_cond} with probability at least $1-\delta_{\text{MS}}$ with $\delta_{\text{MS}} = \delta / T_{\text{MS}}(\varepsilon)$, then
    
    a) after $T$ iterations of Algorithm~\ref{Alg:rest_str_MS} for the case $\mu > 0$ 
    
    b) after $T^{\text{c}}_{\text{MS}}$ iterations of  Algorithm~\ref{alg:MS} for the case $\mu = 0$ 
    
    we obtain that with probability as least $1 - \delta$ we find $\hat{\eta}$ such that $f(\hat{\eta}) - f(\eta^{\ast}) \leq \varepsilon$.
\end{lem}

\subsection{Step 4.}

Before we give the estimates of the number of oracle calls for $h(\cdot)$ and $g(\cdot)$, we will explain how we plan on obtaining them. 

For $h(\cdot)$ we heed to compute the gradient at each step of Algorithm~\ref{alg:gradient_for_composite}, which we run $T_{\text{MS}}(\varepsilon)$ times. Moreover, at each iteration of  Algorithm~\ref{alg:MS} in step~\eqref{MS_step} we compute the gradient of $f(\cdot)$, so we also need to compute the gradient of $h(\cdot)$.

For $g(\cdot)$ we heed to compute the gradient at each step of the inner algorithm $\mathcal{M}_{inn}$, which we run at each iteration of Algorithm~\ref{alg:gradient_for_composite}, and at each iteration of  Algorithm~\ref{alg:MS} in step~\eqref{MS_step} we also need to compute the gradient of $g(\cdot)$.

Note that using the triangle inequality we have 
\begin{equation}
\label{triangl_1}
    ||v^0 - v^{\ast}||_2 \leq ||v^0 - \hat{v}||_2 + ||\hat{v} - v^{\ast}||_2.
\end{equation}
And at each iteration of Algorithm~\ref{alg:gradient_for_composite} we use the method $\mathcal{M}_{inn}$ with starting point $\zeta^k$ to compute the point $\zeta^{k+1}$. So for the $k$-th iteration of Algorithm~\ref{alg:gradient_for_composite} we have $v^0 \equiv \zeta^k$ and $\hat{v} \equiv \zeta^{k+1}$.
Using the triangle inequality and Theorem~\ref{Th:gradient_for_composite}, we have 
\begin{eqnarray*}
    ||\zeta^k - \zeta^{k+1}||_2 \leq ||\zeta^k - \zeta^{\ast}||_2 + ||\zeta^{k+1} - \zeta^{\ast}||_2 \leq 2 \sqrt{\tfrac{L_h}{L}} ||\zeta^0 - \zeta^{\ast}||_2 + 2 \sqrt{\tfrac{2L_h}{L^2}\tilde{\varepsilon}}.
\end{eqnarray*}

Then, using~\eqref{inex_sol_arg}, from~\eqref{triangl_1} we have 
\begin{equation}
      || v^0 - v^{\ast}||_2  \leq  ||v^0 - \hat{v}||_2 + \sqrt{\tilde{\varepsilon} / L_g  }   \leq  \sqrt{\tfrac{4L_h}{L}} ||\zeta^0 - \zeta^{\ast}||_2 + \sqrt{\tilde{\varepsilon}} \left( \sqrt{\tfrac{8L_h}{L^2}} + \sqrt{\tfrac{1}{L_g}  }  \right).
     \label{norm_est}
\end{equation}
   
   Choosing the $\tilde{\varepsilon} = \varepsilon_{\mathcal{M}}$ and using Lemma~\ref{inn_est} we obtain that we need   $N_{\mathcal{M}}(\varepsilon_{\mathcal{M}}) = O\left(\tfrac{\tau_{g}}{\sqrt{L + L_h}}\ln\tfrac{2C L_g ||v^0 - v^{\ast}||_2^2 }{\tilde{\delta}\varepsilon_{\mathcal{M}} (L+L_h)} \right)$ Oracle calls of $\mathcal{M}_{inn}$.
   And using~\eqref{norm_est} we obtain that in $\tilde{N}_{\mathcal{M}} = O\left(\tfrac{\tau_{g}}{\sqrt{L + L_h}} \ln\tfrac{C_1  }{\tilde{\delta}}  \right) \geq N_{\mathcal{M}}(\varepsilon_{\mathcal{M}})$ Oracle calls the Lemma~\ref{inn_est} holds with $\tilde{\varepsilon} = \varepsilon_{\mathcal{M}}$ and $C_1 = \tfrac{2C(32L_h^2 L_g (3L+2L_f)^2 + (8L_h L_g + L^2)L^3}{L^4 (L+L_h)}$.
   
   Each time choosing $\tilde{\delta} \approx  \delta_{\text{MS}}/ N_{\text{GMCO}} = \delta / (N_{\text{GMCO}} \cdot T_{\text{MS}})$ we obtain that we need $N^{\text{SC}}_{\mathcal{M}} = O\left(\tfrac{\tau_{g}}{\sqrt{L + L_h}} \ln\tfrac{C_1 L_h }{\delta \sqrt{\mu L}}  \right)$ Oracle calls of $\mathcal{M}_{inn}$ for the strongly convex case and $N^{\text{C}}_{\mathcal{M}}(\varepsilon) = O\left(\tfrac{\tau_{g}}{\sqrt{L + L_h}} \ln\tfrac{C_1 L_h R}{\delta \sqrt{\varepsilon L}}  \right)$ Oracle calls for the convex case, where $R \geq ||x^0 - x^{\ast}||_2$.

   Using the union bound over all launches of $\mathcal{M}_{inn}$, we obtain that with probability at least $1 - \delta$ we can find such $\hat{x}$ that $f(\hat{x}) - f(x^{\ast}) \leq \varepsilon$, and to do this we need $
   O\left(\sqrt{\tfrac{L}{\mu }} \log\left(\tfrac{  \mu R^2}{\varepsilon} \right) \cdot \left(1 + \tfrac{L_h}{L} \right) \right)
 $
Oracle calls for $h(\cdot)$ and \begin{eqnarray*}
   O \left(\sqrt{\tfrac{L}{\mu}}  \log\left(\tfrac{  \mu R^2}{\varepsilon}\right) \cdot \left(\kappa_g + \tfrac{L_h}{L}\cdot \left(\tfrac{\tau_{g}}{\sqrt{L + L_h}}\ln\tfrac{1}{\delta } \right) \right) \right) 
   \end{eqnarray*}
   Oracle calls for $g(\cdot)$,  if $\mu > 0$,
   
   and 
$
   O\left(\sqrt{\tfrac{LR^2}{\varepsilon}} \cdot \left(1 + \tfrac{L_h}{L} \right) \right)$
Oracle calls for $h(\cdot)$ and 
\begin{eqnarray*}
   O \left(\sqrt{\tfrac{LR^2}{\varepsilon}} \cdot \left(\kappa_g + \tfrac{L_h}{L}\cdot \left(\tfrac{\tau_{g}}{\sqrt{L + L_h}}\ln\tfrac{R}{\delta \sqrt{\varepsilon}} \right) \right) \right) 
   \end{eqnarray*}
   Oracle calls for $g(\cdot)$, if $\mu = 0$.

\section{Proof of the convergence Theorem for the inexact GMCO}\label{GMCO}

\begin{defin}
\label{solNemirovskiy}
For a convex optimization problem 
% \begin{gather}
% \label{Ax_problem}
$\min_{x \in Q} \Psi(x)$,
% \end{gather}
we denote by $\text{Arg}\min_{x \in Q}^{\widetilde{\delta}}\Psi(x)$~a set of such $\widetilde{x}$ that
\begin{gather}\label{eqv_inex_sol}
\exists h \in \partial\Psi(\widetilde{x}):\forall x \in Q \,\, \to\, \left\langle h, x - \widetilde{x} \right\rangle \geq -\widetilde{\delta}.
% ,\,\,\, \forall x \in Q.
\end{gather}
We denote by $\argmin_{x \in Q}^{\widetilde{\delta}}\Psi(x)$  some element of $\text{Arg}\min_{x \in Q}^{\widetilde{\delta}}\Psi(x)$.
\end{defin}

\begin{algorithm}[ht]
	\caption{Gradient method for Composite Optimization $\text{GMCO}(x_0, F(\cdot))$}
	\begin{algorithmic}[1]
		\STATE {\bf Parameters:} starting point $x_0 \in \mathbb{R}^n$, objective function $F(x) = f(x) + p(x)$, constant $L$ (function $f$ with $L$ Lipschitz gradient w.r.t. the $||\cdot||_2$), error $\widetilde{\delta}$.
		\FOR{$k = 0, \ldots,N-1$}
			\STATE Set
			\begin{align*}
			\phi_{k+1}(x) := \left\langle \nabla f(x_k), x - x_k \right\rangle + p(x) + \tfrac{L}{2} \|x - x_k\|_2^2,
			\end{align*}
			\STATE Compute 
			\begin{equation}
			\label{alg:gradient_for_composite_base:auxilary}
			   x_{k+1}:={\argmin_{x \in Q}}^{\widetilde{\delta}}(\phi_{k+1}(x))
			\end{equation}
		\ENDFOR
		\STATE {\bf Output:} $x_N$
	\end{algorithmic}
	\label{alg:gradient_for_composite_base}
\end{algorithm}

\begin{lem}
    \label{lemma:str_conv}
	Let $\psi(x)$ be a convex function and
	\begin{gather*}
	y = {\argmin_{x \in Q}}^{\widetilde{\delta}} \left\lbrace \psi(x) + \tfrac{\beta}{2}||z - x||^2_2\right\rbrace,
	\end{gather*}
	where $\beta \geq 0$.
Then
	\begin{align*}
\psi(x) + \tfrac{\beta}{2}||z - x||^2_2
\geq \psi(y) + \tfrac{\beta}{2}||z - y||^2_2 + \tfrac{\beta}{2}||x - y||^2_2 - \widetilde{\delta} ,\,\,\, \forall x \in Q.
	\end{align*}
\end{lem}

\begin{proof}
    By Definition \ref{solNemirovskiy}:
    \begin{gather*}
		\exists g \in \partial\psi(y), \,\,\, \left\langle g + \tfrac{\beta}{2} \nabla_y ||y - x||^2_2, x - y \right\rangle = \left\langle g + \beta(y - z), x - y \right\rangle \geq -\widetilde{\delta} ,\,\,\, \forall x \in Q.
	\end{gather*}
    From $\beta$--strong convexity of $\psi(x) + \tfrac{\beta}{2}||z - x||^2_2$ we have
    \begin{gather*}
		\psi(x) + \tfrac{\beta}{2}||z - x||^2_2 \geq \psi(y) + \tfrac{\beta}{2}||z - y||^2_2 + \left\langle g + \tfrac{\beta}{2} \nabla_y ||y - x||^2_2, x - y\right\rangle + \tfrac{\beta}{2}||x - y||^2_2
	\end{gather*}
	The last two inequalities complete the proof.
\end{proof}

The next theorem proves convergence rate of Algorithm \ref{alg:gradient_for_composite_base} for optimization problem

\begin{equation}
    \min_{x \in \mathbb{R}^n} F(x):= f(x) + p(x),
\end{equation}

where function $f$ is convex function with $L$-Lipschitz gradient w.r.t. the $||\cdot||_2$ norm, function $p$ is convex function and function $F$ is $\mu$--strongly convex.

\begin{theorem}\label{Th:str_conv_adap}
Let us assume that $\frac{\mu}{2L} \leq 1$. After $N$ iterations of Algorithm \ref{alg:gradient_for_composite_base} we have
\begin{align*}
F(x_{N}) - F(x^{\ast}) \leq \exp\left(-\frac{N\mu}{4L}\right) (F(x_{0}) - F(x^{\ast})) + \frac{4L}{\mu}\widetilde{\delta},
\end{align*}
\begin{align*}
    \frac{1}{2}||x^{\ast} - x_{N}||^2_2 \leq \frac{L}{2\mu} ||x^{\ast} - x_{0}||^2_2 + \frac{4L}{\mu^2}\widetilde{\delta}.
\end{align*}
\end{theorem}

%\begin{proof}[Proof of Theorem \ref{Th:str_conv_adap}] 
{\it Proof}
Since gradient of function $F$ is $L$-Lipschitz w.r.t. the $||\cdot||_2$ norm, we have
\begin{align*}
F(x_{N}) \leq  f(x_{N-1}) + \left\langle \nabla f(x_{N-1}), x_{N} - x_{N-1} \right\rangle + p(x_N) + \frac{L}{2}||x_{N-1} - x_{N}||^2_2.
\end{align*}
From Lemma \ref{lemma:str_conv} and auxiliary problem \eqref{alg:gradient_for_composite_base:auxilary} we get
\begin{align*}
F(x_{N})
\leq f(x_{N-1}) +\left\langle \nabla f(x_{N-1}), x - x_{N-1} \right\rangle + p(x) + \frac{L}{2}||x - x_{N-1}||^2_2 + \widetilde{\delta}.
\end{align*}
In view of convexity of function $f$, we obtain
\begin{align}
\label{analysis_algorithm_grad:prove_1}
F(x_{N}) \leq F(x) + \frac{L}{2}||x - x_{N-1}||^2_2 + \widetilde{\delta}.
\end{align}
We rewrite the last inequality for $x = \alpha x^{\ast} + (1 - \alpha) x_{N-1}$ ($\alpha \in [0, 1]$) as
\begin{align*}
F(x_{N}) \leq F( \alpha x^{\ast} + (1 - \alpha) x_{N-1}) + \frac{L\alpha^2}{2}||x^{\ast} - x_{N-1}||^2_2 + \widetilde{\delta}.
\end{align*}
In view of convexity of function $f$, we have
\begin{align*}
F(x_{N}) \leq F(x_{N-1}) -\alpha (F(x_{N-1}) - F(x^{\ast})) + \frac{L\alpha^2}{2}||x^{\ast} - x_{N-1}||^2_2 + \widetilde{\delta}.
\end{align*}
From $\mu$--strong convexity of function $F$ we have $F(x_{N-1}) \geq F(x^{\ast}) + \frac{\mu}{2}||x^{\ast} - x_{N-1}||^2_2$, this yields inequality:
\begin{align*}
F(x_{N}) \leq F(x_{N-1}) -\alpha \left(1 - \alpha\frac{L}{\mu}\right) (F(x_{N-1}) - F(x^{\ast})) + \widetilde{\delta}.
\end{align*}
The minimum of the right part of the last inequality is achieved with $\alpha = \min(1, \frac{\mu}{2L})$. Due to $\frac{\mu}{2L} \leq 1$ with $\alpha = \frac{\mu}{2L}$ we have
\begin{align*}
F(x_{N}) - F(x^{\ast}) \leq \left(1 - \frac{\mu}{4L}\right) (F(x_{N-1}) - F(x^{\ast})) + \widetilde{\delta}.
\end{align*}
and
\begin{align*}
F(x_{N}) - F(x^{\ast}) &\leq \left(1 - \frac{\mu}{4L}\right)^N (F(x_{0}) - F(x^{\ast})) + \frac{4L}{\mu}\widetilde{\delta}\\
&\leq \exp\left(-\frac{N\mu}{4L}\right) (F(x_{0}) - F(x^{\ast})) + \frac{4L}{\mu}\widetilde{\delta}.
\end{align*}
From $\mu$--strong convexity of function $F$ and the fact that gradient of function $F$ is $L$ Lipschitz we obtain
\begin{align*}
    \frac{1}{2}||x^{\ast} - x_{N}||^2_2 &\leq \frac{L}{2\mu} \exp\left(-\frac{N\mu}{4L}\right) ||x^{\ast} - x_{0}||^2_2 + \frac{4L}{\mu^2}\widetilde{\delta}\\
    &\leq \frac{L}{2\mu} ||x^{\ast} - x_{0}||^2_2 + \frac{4L}{\mu^2}\widetilde{\delta}.
\end{align*}
%\end{proof}
\qed
